# Supplementary material for: Intrinsic coercivity induced by valence fluctuations in $4f$-$3d$ intermetallic magnets
Source: arXiv:2103.10202 source file (2021-03-18)
Supplement: Supplementary file 1 [file CeCoCu5_SI.pdf]

# Supplementary Material for
# "Intrinsic coercivity induced by valence fluctuations in $4f$-$3d$ intermetallic magnets"

Hiroaki Shishido[1], Tetsuro Ueno[2], Kotaro Saito[3], Masahiro Sawada[4], and Munehisa Matsumoto[5*]
[1] *Department of Physics and Electronics, Osaka Prefecture University, 1-1 Gakuen-cho, Naka-ku, Sakai, Osaka 599-8531, Japan*
[2] *Quantum Beam Science Research Directorate, National Institutes for Quantum and Radiological Science and Technology, 1-1-1 Kouto, Sayo, Hyogo 679-5148, Japan*
[3] *Institute of Materials Structure Science, High Energy Accelerator Research Organization, 1-1 Oho, Tsukuba, Ibaraki 305-0801, Japan*
[4] *Hiroshima Synchrotron Radiation Center, Hiroshima University, Higashi-Hiroshima, Hiroshima 739-0046, Japan*
[5] *Institute for Solid State Physics (ISSP), University of Tokyo, Kashiwa 277-8581, Japan*
(Dated: March 18, 2021)

In this supplementary Material, we show the crystal structure of the target materials, Ce(Co,Cu)$_5$, all of the measured magnetization curves that was not high-lighted in the main text, the minor temperature dependence of the XAS data, and the setup of the electronic structure calculations including the choice of the parameter $U_{3d}$.

## S1. THE CRYSTAL STRUCTURE

The crystal structure of Ce(Co,Cu)$_5$ is depicted in Fig. S1. Cu replaces Co in both of the Co($2c$) and Co($3g$) sublattices with some preference for the Co($2c$) sites [S1].

## S2. MAGNETIZATION CURVES FOR ALL SAMPLES

In the main text, we highlighted the emergence of intrinsic coercivity in the intermediate concentration range of Cu in Ce(Co,Cu)$_5$. Here other measured magnetization curves with less significant coercivity are presented in Figs. S2 and S3 to complete the description of what we investigated. Magnetization curves for Ce(Co$_{1-x}$Cu$_x$)$_5$ ($x < 0.6$) exhibit ferromagentic features clearly, while those for Ce(Co$_{0.3}$Cu$_{0.7}$)$_5$ exhibit paramagnetic field dependence. The magnetism trend with respect to $x$ is consistent with what was reported in the previous work [S3] in that the Curie temperature of 650 K at $x = 0$ decreases with $x$ and disappears around $x = 0.6$.

## S3. THE MINOR TEMPERATURE DEPENDENCE OF THE XAS DATA

In the main text we presented the XAS data at 20 K since the temperature dependence was minor as compared to the $x$-dependence of Ce(Co$_{1-x}$Cu$_x$)$_5$. The details of the way how the temperature dependence is minor is shown

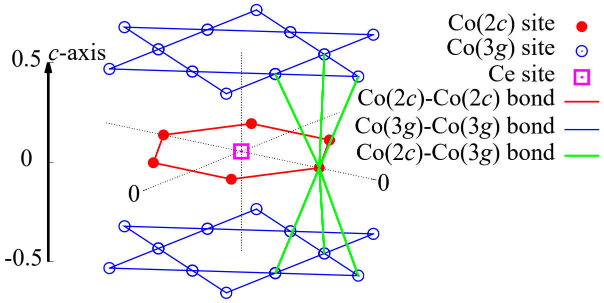


FIG. S1. Crystal structure of Ce(Co,Cu)$_5$ which is isostructural to YCo$_5$ as seen in Ref. S2.

---

* Present address: Institute of Materials Structure Science, High Energy Accelerator Research Organization (KEK), 1-1 Oho, Tsukuba, Ibaraki 305-0801, Japan

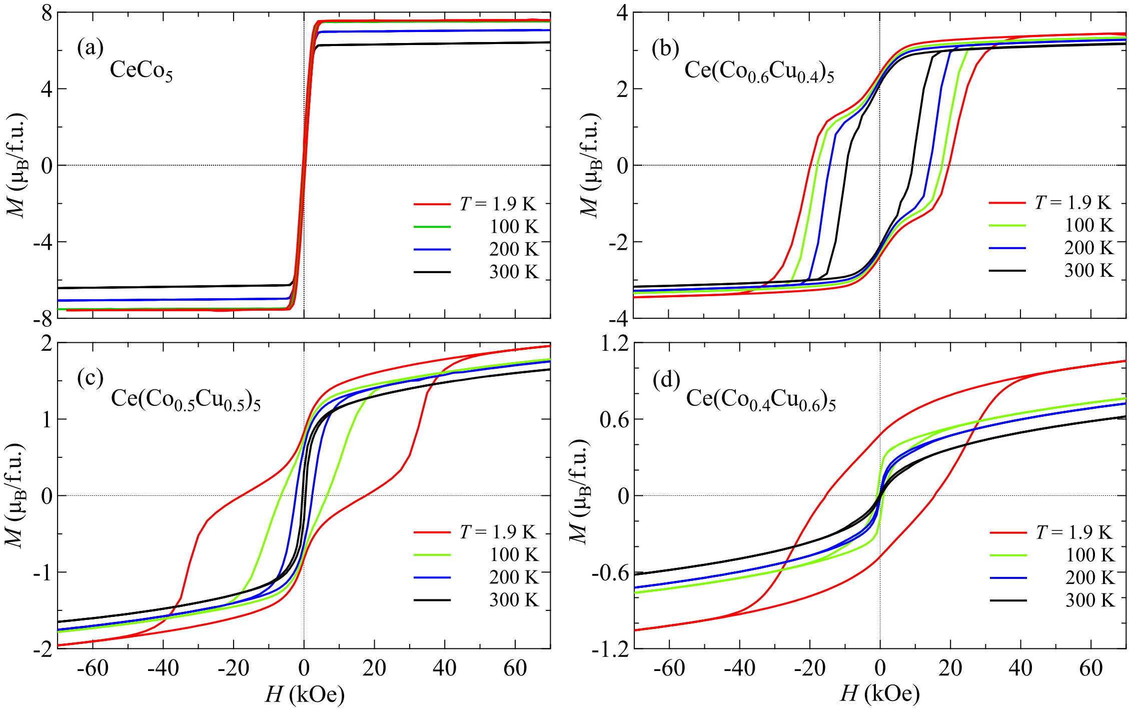


FIG. S2. (Color online) Magnetization curves of $Ce(Co_{1-x}Cu_x)_5$ for (a) $x = 0$ (b) 0.4, (c) 0.5 , and (d) 0.6 at the temperatures of 300 K, 200 K, 100 K, and 1.9 K.

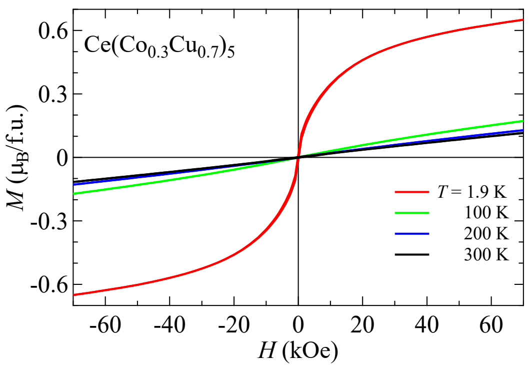


FIG. S3. (Color online) Magnetization curves of $Ce(Co_{0.3}Cu_{0.7})_5$ at the same temperature range as Fig. S2.

in Fig. S4. The XAS data is virtually temperature independent, indicating that the observed mixed valence state persists from 20 K to the higher temperatures to 300 K. On the more Cu-enriched compounds, enhancement of the localization of the $4f$ electron in the ground state would bring about the Kondo effect. Detailed investigations on these aspects are reported separately [S4].

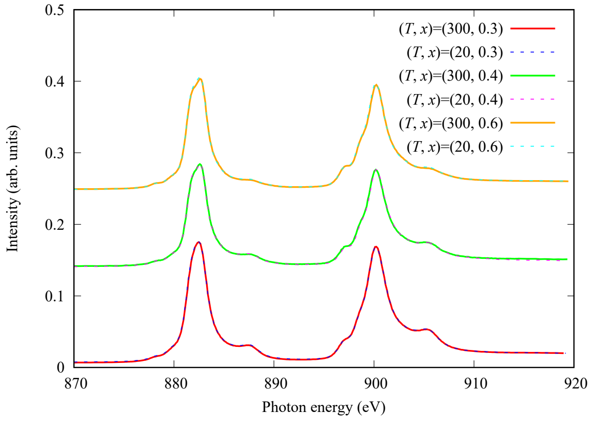


FIG. S4. (Color online) Measured XAS spectra of $Ce(Co_{1-x}Cu_x)_5$ for $x = 0.3$ $x = 0.4$, and $x = 0.6$. We see virtually no temperature dependence.

## S4. THE PRESENT CALCULATION SCHEME, ITS SCOPE, AND BEYOND

### A. Computational setup with *OpenMX*

We give the details of the computational setup using *OpenMX* [S5–S10] for the electronic structure calculations. Calculations with *OpenMX* are based on the linear combination of pseudo-atomic orbitals and fully relativistic pseudopotentials [S11, S12]. Proper choice of the local basis sets is crucial to reach the reliable conclusions. We used the $k$-space mesh of $8 \times 8 \times 8$ and the local basis sets of `Ce8.0-s3p3d3f2` and `Co6.0S-s2p2d2f1` for Ce and Co, respectively. Here the numbers after the name of the element indicates the cutoff radii in bohr and the numbers after the name of the orbitals, $s$, $p$, $d$, and $f$, are the number of orbitals included in the calculation. For the structure optimization and the calculation of magnetic anisotropy based in the optimized lattice, we used the generalized gradient approximation (GGA) according to Perdew, Burke, and Enzerhof [S13].

### B. Rationale for setting $U_{3d} = 2eV$

The $3d$-electron part in the magnetism of $RCo_5$ (R=rare earth) has often been described with a case study on $YCo_5$ [S1, S2]. Here we also employ such approaches and follow the same procedure as we do for $CeCo_5$ in the main text. That is, we start with the experimental lattice, do the structure optimization and then calculate the magnetic moments with DFT+U by varying $U_{3d} = 0$ to 2.5 (eV) for the $3d$-electrons in Co. Calculated results for the spin magnetic moment and orbital magnetic moment are shown in Fig. S5 (a) and (b), respectively. While the overall trend of the calculated spin moments are slightly overestimated as has been known to be the case generally with GGA, the trends of the calculated orbital moments with respect to $U_{3d}$ can be referred to select the realistic parameter range for $U_{3d}$. We see that the calculated orbital moments come closest to the experimental values around $U_{3d} = 2$ (eV). Even though an exact match between the past experimental report [S14] and our present calculations is never observed, which is reasonable considering the possible systematic deviations on both of experiments and calculations, we conclude that $U_{3d} = 2$ (eV) seems to be in the good working range with which the experimental energy scale concerning the $3d$-electron magnetism is most realistically described.

### C. The scope of the present calculations and beyond

In the present work, we have applied the DFT+U method following Ref. [S15] to demonstrate the anomalous magnetic anisotropy triggered by the valence fluctuations in Ce. Here combination of SOI and the charge transfer process between the $4f$-electron of Ce and $3d$-electrons of Co working in the energy scale of $O(0.1)$ (eV) in the direct $4f$-$3d$ hybridization is the crucial part to bring about an order of enhancement in the effective magnetic anisotropy, as compared to the conventional one realized by the combination of SOI and crystal fields, amounting to $O(10)$ (meV). In order to focus on the effects of the valence fluctuation, we have shown the results with respect to the $U_{4f}$ in

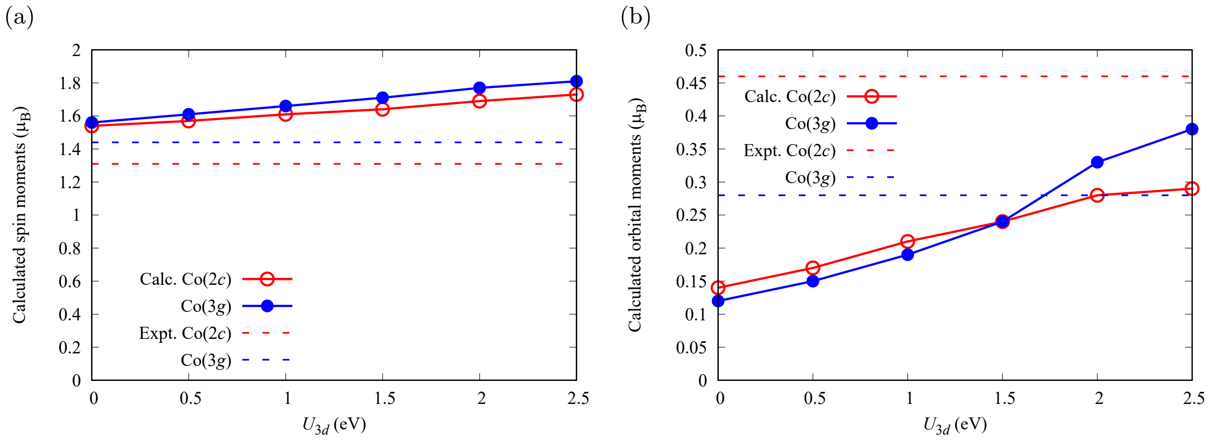


FIG. S5. (Color online) Calculated magnetic moments of $YCo_5$. (a) spin components and (b) orbital components are separately shown. Experimental data are taken from Ref S14 as a reference.

$CeCo_5$ that controls the degree how the $4f$-electrons are relatively localized. In reality, the effects of Cu substitution obviously dilutes the $3d$-electron magnetization and associated changes in the lattice constants also modified the electronic structure. Those effects should come in in the next leading order or in the higher orders to impose some corrections to the calculated results.

While the Hartree-Fock solution in DFT+U should be able to describe the trends in the energy and the intrinsic magnetism to the leading order, it is of more theoretical interest to inspect the contribution from off-diagonal component in the $c$-$f$ hybridization and the more refined solution of the associated quantum many-body problem [S16]. Such refinement would be crucial in addressing the low-temperature magnetic anisotropy, which may be analogously described for some U-based ferromagnets. Further developments along this line are in progress.

[S1] K. Uebayashi, K. Terao, and H. Yamada, J. Alloys Compds. **346**, 47 (2002).
[S2] M. Matsumoto, R. Banerjee, J. B. Staunton, Phys. Rev. B **90**, 054421 (2014).
[S3] D. Girodin, C. H. Allibert, F. Givord, R. Lemaire, J. Less Common Metals **110**, 149 (1985).
[S4] Part of the results on the Cu-rich side of $Ce(Co,Cu)_5$ within a Kondo lattice model based on the realistic electronic structure is reported in M. Matsumoto, Phys. Rev. Mater. **4**, 054401 (2020).
[S5] the source code is available at the following website: `http://www.openmx-square.org/`
[S6] T. Ozaki, Phys. Rev. B. **67**, 155108 (2003).
[S7] T. Ozaki and H. Kino, Phys. Rev. B **69**, 195113 (2004).
[S8] T. Ozaki and H. Kino, Phys. Rev. B **72**, 045121 (2005).
[S9] T. V. T. Duy and T. Ozaki, Comput. Phys. Commun. **185**, 777 (2014).
[S10] K. Lejaeghere *et al.*, Science **351**, aad3000 (2016).
[S11] I. Morrison, D.M. Bylander, L. Kleinman, Phys. Rev. B **47**, 6728 (1993).
[S12] G. Theurich and N.A. Hill, Phys. Rev. B **64**, 073106 (2001).
[S13] J. P. Perdew, K. Burke, and M. Ernzerhof, Phys. Rev. Lett. **77**, 3865 (1996).
[S14] J. Schweizer and F. Tasset, J. Phys. F: Met. Phys. **10**, 2799 (1980).
[S15] M.-J. Han, T. Ozaki, J. Yu, Phys. Rev. B **73**, 045110 (2006).
[S16] For a review, see e.g. H. Shinaoka, Y. Motome, T. Miyake, S. Ishibashi, P. Werner, J. Phys.: Condens. Matter **31**, 323001 (2019).
